# Supplementary material for: Domain-Specific Block Selection and Paired-View Pseudo-Labeling for Online Test-Time Adaptation
Source: arXiv:2404.10966 source file (2024-05-07)
Supplement: Supplementary file 1 [file X_suppl.tex]

\clearpage
\setcounter{page}{1}
\maketitlesupplementary

% % 
% Having the supplementary compiled together with the main paper means that:
% % 
% \begin{itemize}
% \item The supplementary can back-reference sections of the main paper, for example, we can refer to \cref{sec:intro};
% \item The main paper can forward reference sub-sections within the supplementary explicitly (e.g. referring to a particular experiment); 
% \item When submitted to arXiv, the supplementary will already included at the end of the paper.
% \end{itemize}
% % 
% To split the supplementary pages from the main paper, you can use \href{https://support.apple.com/en-ca/guide/preview/prvw11793/mac#:~:text=Delete%20a%20page%20from%20a,or%20choose%20Edit%20%3E%20Delete).}{Preview (on macOS)}, \href{https://www.adobe.com/acrobat/how-to/delete-pages-from-pdf.html#:~:text=Choose%20%E2%80%9CTools%E2%80%9D%20%3E%20%E2%80%9COrganize,or%20pages%20from%20the%20file.}{Adobe Acrobat} (on all OSs), as well as \href{https://superuser.com/questions/517986/is-it-possible-to-delete-some-pages-of-a-pdf-document}{command line tools}.

\section*{Architectures}
Here, we describe the details of each architecture used in the experiments. All source pre-trained weights are provided by RobustBench\cite{croce2020robustbench}.
\begin{itemize}
    \item WRN28-10. We use a wide residual network \cite{Zagoruyko2016WRN} with a depth of 28 and a width of 10. Additionally, the network has 12 residual blocks.
    \item WRN40-2A. We use a wide residual network with a depth of 40 and a width of 2. This network is trained using AugMix \cite{hendrycks2020augmix}, a data processing technique that improves the model for unseen corruptions. The network has 18 residual blocks.
    \item ResNet-18A. We use a residual network with 18 layers trained by adversarial training to improve robustness against corruptions \cite{kireev2022effectiveness}. The network has 8 residual blocks.
    \item ResNext-29A. We use ResNext\cite{xie2017aggregated} with 29 layers. ResNext improves ResNet architecture by employing cardinality from group convolution. The network is trained with AugMix \cite{hendrycks2020augmix} augmentation by SGD optimizer using an initial learning rate of 0.1, which decays following a cosine learning rate and is trained for 200 epochs. The network has 9 blocks.
    \item ResNet50. We use a residual network with 50 layers for the ImageNet benchmark. The network has 16 blocks.
    \item ResNet50A. We also use a residual network with 50 layers trained using AugMix for the ImageNet benchmark. The network has 16 blocks.
    
\end{itemize}

\begin{table*}[t!]
\centering
\resizebox{0.9\textwidth}{!}{
\begin{tabular}{llccccccccccccccccc}
\hline
\multicolumn{1}{c}{}                                & \multicolumn{18}{c}{Blocks}                                                                                                                                                                                                                                                                                                                                                                                                 \\ \cline{2-19} 
\multicolumn{1}{c}{\multirow{-2}{*}{Architectures}} & 1                            & 2                            & 3                            & 4                            & 5                            & 6                            & 7                            & 8                            & 9                            & 10                           & 11                           & 12                           & 13   & 14   & 15   & 16   & 17   & 18   \\ \hline
\multicolumn{1}{l|}{WRN28-10}                       & \cellcolor[HTML]{C0C0C0}0.89 & \cellcolor[HTML]{C0C0C0}0.92 & \cellcolor[HTML]{C0C0C0}1.0  & \cellcolor[HTML]{C0C0C0}0.98 & 0.49                         & 0.47                         & 0.54                         & 0.49                         & 0.30                         & 0.20                         & 0.09                         & 0.0                          & -    & -    & -    & -    & -    & -    \\
\multicolumn{1}{l|}{WRN40-2A}                       & \cellcolor[HTML]{C0C0C0}0.99 & \cellcolor[HTML]{C0C0C0}1.0  & \cellcolor[HTML]{C0C0C0}1.0  & \cellcolor[HTML]{C0C0C0}0.99 & \cellcolor[HTML]{C0C0C0}1.0  & \cellcolor[HTML]{C0C0C0}1.0  & \cellcolor[HTML]{C0C0C0}0.9  & \cellcolor[HTML]{C0C0C0}0.76 & \cellcolor[HTML]{C0C0C0}0.85 & \cellcolor[HTML]{C0C0C0}0.78 & \cellcolor[HTML]{C0C0C0}0.80 & \cellcolor[HTML]{C0C0C0}0.86 & 0.34 & 0.59 & 0.45 & 0.0  & 0.43 & 0.14 \\
\multicolumn{1}{l|}{ResNet18A}                      & \cellcolor[HTML]{C0C0C0}0.93 & \cellcolor[HTML]{C0C0C0}1.0  & 0.58                         & 0.53                         & 0.29                         & 0.37                         & 0.26                         & 0.0                          & -                            & -                            & -                            & -                            & -    & -    & -    & -    & -    & -    \\
\multicolumn{1}{l|}{ResNext-29}                     & \cellcolor[HTML]{C0C0C0}0.91 & \cellcolor[HTML]{C0C0C0}1.0  & \cellcolor[HTML]{C0C0C0}0.97 & 0.67                         & 0.67                         & 0.59                         & 0.34                         & 0.39                         & 0.0                          & -                            & -                            & -                            & -    & -    & -    & -    & -    & -    \\
\multicolumn{1}{l|}{WRN40-2A}                       & \cellcolor[HTML]{C0C0C0}0.95 & \cellcolor[HTML]{C0C0C0}0.96 & \cellcolor[HTML]{C0C0C0}0.97 & \cellcolor[HTML]{C0C0C0}0.99 & \cellcolor[HTML]{C0C0C0}1.0  & \cellcolor[HTML]{C0C0C0}1.0  & \cellcolor[HTML]{C0C0C0}0.80 & 0.71                         & 0.72                         & 0.69                         & 0.70                         & 0.69                         & 0.28 & 0.38 & 0.31 & 0.27 & 0.20 & 0.0  \\
\multicolumn{1}{l|}{ResNet50}                       & \cellcolor[HTML]{C0C0C0}0.96 & \cellcolor[HTML]{C0C0C0}1.0  & \cellcolor[HTML]{C0C0C0}0.95 & 0.38                         & 0.57                         & 0.52                         & 0.51                         & 0.31                         & 0.58                         & 0.54                         & 0.48                         & 0.46                         & 0.43 & 0.0  & 0.26 & 0.12 & -    & -    \\
\multicolumn{1}{l|}{ResNet50A}                      & \cellcolor[HTML]{C0C0C0}0.99 & \cellcolor[HTML]{C0C0C0}1.0  & \cellcolor[HTML]{C0C0C0}1.0  & \cellcolor[HTML]{C0C0C0}1.0  & \cellcolor[HTML]{C0C0C0}0.97 & \cellcolor[HTML]{C0C0C0}0.99 & \cellcolor[HTML]{C0C0C0}1.0  & 0.47                         & 0.54                         & 0.53                         & 0.41                         & 0.48                         & 0.48 & 0.24 & 0.23 & 0.0  & -    & -    \\ \hline
\end{tabular}}
\caption{Block selection results. The block with grey background color refers to the selected block as it has larger value than 0.75. Architectures in 1-3rd row, 4-5th row, and 6-7th row are for CIFAR10-C, CIFAR100-C, and ImageNet-C, respectively.}
\label{tab:blockselectionresult}
\end{table*}

\section*{Details of the baselines}
Also, we describe the details of each baseline used in the experiments.
\begin{itemize}
    \item Source only. It is a baseline method that does not use any test-time adaptation method. Thus, it represents the performance of the source pre-trained model directly used in shifted domains.
    \item BN-1 \cite{nado2020evaluating, schneider2020improving}. BN-1 is a simple method that recalculates the batch normalization statistics using the current test batch.
    \item TENT-cont. \cite{wang2021tent}. It is an entropy minimization-based method where weights of the batch normalization layer in the network are updated to minimize the entropy of current prediction as follows.
    \begin{equation}
        \mathcal{L}_{en} = -\sum_c \hat{y}_c \log \hat{y}_c.
    \end{equation}
    
    \item AdaContrast \cite{chen2022contrastive}. This is a test-time adaptation method based on the contrastive learning.  It uses self-training with pseudo-labels along with contrastive learning, enabling discriminative feature learning by pulling positive pairs closer and pushing negative pairs away. The paired images are generated using weak and strong augmentations.
    \item CoTTA \cite{wang2022continual}. It is a test-time adaptation framework that works in a continually changing environment based on consistency regularization. This framework uses the teacher's augmentation-averaged pseudo-label, generated by averaging predictions for 32 augmented images, to train the student. Also, it employs stochastic restore, which restores the current weight to the original source pre-trained weight, to reduce error accumulation.
    \item EATA \cite{niu2022efficient}. It is an improved version of TENT that uses reliable sample selection. Specifically, they investigate the sample that makes model collapse and find that high-entropy samples are reason. Therefore, they only use low-entropy samples to update the weight parameters of batch normalization by entropy minimization during test-time as follows.
        \begin{equation}
            S^{ent}(x) = \frac{1}{\exp[E(x;\theta)-E_0]} \cdot \mathbb{I}_{\{E(x;\theta)<E_0\}}(x),
        \end{equation}
    where $\mathbb{I}_{\{\cdot\}}(\cdot)$ is an indicator function, $E(x;\theta)$ is the entropy of a given sample $x$. Also, $E_0$ is a threshold. It excludes high-entropy samples and assigns higher weights to low-entropy samples. Moreover, it utilizes Fisher regularize to alleviate the catastrophic forgetting issue by preventing model parameters, important for source knowledge, from changing too much.
    \item SAR \cite{niu2023towards}. It is also based on the entropy minimization-based method. Specifically, it proposes reliable and sharpness-aware entropy minimization, which selects low-entropy samples and encourages the model to go to a flat area of the loss surface to further achieve good generalization ability. Also, it provides a model recovery scheme based on the insight that models after collapse will produce very small entropy loss. This method is based on Group Norm and Layer Norm but can apply to Batch Norm networks as well.
    \item RMT \cite{dobler2023robust}. RMT is a consistency regularization-based method where the student model is trained by pseudo-labels generated by EMA teacher. The student model has two losses: symmetric cross-entropy between student's prediction and teacher's prediction. It also utilizes contrastive loss that pulls current test features towards source feature space. It uses source replays to further use source training data in test-time, but we do not compare our method to this result since it is not source-free.
\end{itemize}

\section*{Domain-specific block selection results}

In Table \ref{tab:blockselectionresult}, we present the specific results of the block selection. As mentioned in Section \ref{sec:experiment}, we use WRN28-10, WRN40-2A, and ResNet18A for CIFAR10-C. Additionally, we employ ResNext-29A and WRN40-2A for CIFAR100-C. Finally, we utilize ResNet50 and ResNet50A for ImageNet-C.

We observed that shallow blocks tend to exhibit high similarity, whereas deeper blocks tend to show smaller similarity. In the experiment, we select blocks with a similarity higher than 0.75. For instance, we choose 1-4 blocks when using the WRN28-10 architecture, and 1-2 blocks when using ResNet18A.

\section*{Computational time}
Since our framework updates the parameters twice for a given batch, the computational time can be burdensome for real-time systems. Despite that, our framework uses only one augmentation (i.e., horizontal flip) for generating pseudo-labels, which is much lighter than CoTTA's 32 augmentations. In Table \ref{tab:time}, we provide the computational time when using ResNext-29 for CIFAR100-C. All computational times are averaged over 15,000 batches. Our test setting is based on PyTorch 2.0.1, RTX 4090 GPU, and Linux 20.04. Our method has a relatively large computational time compared to other methods, which may be a limitation.

\begin{table}[h]
\centering
\resizebox{0.3\textwidth}{!}{
\begin{tabular}{@{}l|cc@{}}
\toprule
\multirow{2}{*}{Method} & \multicolumn{2}{c}{Architectures} \\ \cmidrule(l){2-3} 
                        & WRN28-10       & ResNext-29A       \\ \midrule
Source                  & 45.3           & 29.0             \\
BN-1                    & 46.2           & 31.3             \\
TENT                    & 96.8           & 70.9             \\
AdaContrast             & 315.1          & 200.7            \\
CoTTA                   & 842.9          & 806.3            \\
EATA                    & 98.5           & 73.5             \\
SAR                     & 189.8          & 137.6            \\
RMT                     & 322.1          & 203.0            \\
DPLOT (ours)            & 534.0          & 336.7            \\ \bottomrule
\end{tabular}}
\caption{Computational time (ms) to predict and adaptation of a single batch with various methods.}
\label{tab:time}
\end{table}

\section*{Performance at the similar computational time}
We present the adaptation performance, utilizing a similar computational time across various methods in Table \ref{tab:samecost}, to demonstrate the effectiveness of each method while considering the computational burden. To ensure all methods have similar computational time, we modify the number of updates for each method during the test-time stage. Specifically, we adopt the setting of single sample TTA as described in Section \ref{subsec:ssta}, using a buffer size $b$ of 64. Subsequently, we adjust the update frequency $k$ to decrease computational time by reducing adaptation. With $k$, the model parameters are updated using a batch of size $b$ for every $b \times k$ steps. For example, when using $b = 64$ and $k = 1/4$, the model parameters are updated using the last 64 samples every 254 steps. This reduction in adaptation significantly decreases computational time. We decrease the learning rate by $\textit{original batch size}/(b \times k)$ and set $k$ to achieve a computational time of around 200 ms. We did not modify the entropy minimization-based methods, as they already require computational times below 200 ms.

As shown in Table \ref{tab:samecost}, our method still outperforms other methods with a similar computational cost for the CIFAR100-C gradual benchmark. It demonstrated that our method provides relatively strong adaptation performance, even when we adapt the model using our method only once for every six batches.

\begin{table}[ht]
\centering
\resizebox{0.48\textwidth}{!}{
\begin{tabular}{@{}l|ccc@{}}
\toprule
\multicolumn{1}{c|}{Method} & Error rates & Update Frequency & Computational Cost \\ \midrule
TENT                        & 74.2        & 1    & 158                \\
EATA                        & 33.6        & 1    & 198                \\
SAR                         & 33.7        & 1    & 317                \\
AdaContrast                 & 43.8        & 1/3    & 290                \\
CoTTA                       & 44.9        & 1/10    & 229                \\
RMT                         & 31.1        & 1/3    & 211                \\
DPLOT (ours)                & \textbf{26.8}        & 1/6    & 209                \\ \bottomrule
\end{tabular}}
\caption{Classification error rate (\%; @level 1-5) for the CIFAR100-C gradual benchmark with ResNext-29A architecture.}
\label{tab:samecost}
\end{table}

\section*{Performance on mixed domain shifts setting}
We also present experimental results in a mixed domain setting, as in SAR\cite{niu2023towards}, where all kinds corruptions are given to test images simultaneously. Specifically, test data from 15 corruption-type domains are given to the model concurrently. In this setting, the challenge lies in adapting the TTA framework to a model facing multiple domains which have diverse feature statistics. As depicted in Table \ref{tab:mixed}, our method outperforms other methods across various architectures, except for ResNext-29A. We believe that entropy minimization on domain-specific block is also effective in adjusting domain-specific feature extraction, not only for a single corruption but also for a mixture of given corruptions.

\begin{table}[ht]
\centering
\resizebox{0.48\textwidth}{!}{
\begin{tabular}{@{}l|ccccc@{}}
\toprule
\multirow{2}{*}{Method} & \multicolumn{5}{c}{Architectures}                                                                  \\ \cmidrule(l){2-6} 
                        & WRN28-10      & WRN40-2A      & \multicolumn{1}{c|}{ResNet18A}     & ResNext-29A    & WRN40-2A      \\ \midrule
Source                  & 43.5          & 18.3          & \multicolumn{1}{c|}{16.7}          & 46.5          & 46.7          \\
BN-1                    & 33.8          & 20.2          & \multicolumn{1}{c|}{19.4}          & 45.8          & 47.7          \\
TENT                    & 37.2          & 16.6          & \multicolumn{1}{c|}{18.5}          & 84.3          & 56.2          \\
AdaContrast             & 26.1          & 15.0          & \multicolumn{1}{c|}{14.0}          & 41.9          & 42.6          \\
CoTTA                   & 32.3          & 16.7          & \multicolumn{1}{c|}{15.7}          & 43.1          & 46.9          \\
EATA                    & 27.9          & 14.9          & \multicolumn{1}{c|}{14.4}          & \textbf{37.5} & 41.0          \\
SAR                     & 33.7          & 19.9          & \multicolumn{1}{c|}{19.4}          & 45.2          & 42.3          \\
RMT                     & 26.9          & 15.2          & \multicolumn{1}{c|}{13.8}          & 38.4          & 41.9          \\
DPLOT (ours)            & \textbf{24.3} & \textbf{13.0} & \multicolumn{1}{c|}{\textbf{11.9}} & 38.4          & \textbf{38.8} \\ \bottomrule
\end{tabular}}
\caption{Classification error rate (\%) for CIFAR10-C and CIFAR100-C with the mixed domain shifts setting. We use WRN28, WRN40-2A, and ResNet18A for CIFAR10-C benchmark, while ResNext-29A and WRN40-2A are used for CIFAR100-C benchmarks.}
\label{tab:mixed}
\end{table}

\section*{Various corruption settings for block selection}
We present the block selection results with different corruption settings for source training images in Table \ref{tab:corrupt}. In the main experiments, we select the block that has a similarity larger than 0.75 after entropy minimization with Gaussian noise (0.0 $\mu$ and 0.5 $\sigma$) added to source training images. To investigate the effect of corruption on block selection, we vary the Gaussian noise setting. For example, we change the $\sigma$ to 0.1 or 1.0. Additionally, we calculate the similarity with source training images after changing brightness or contrast (i.e., twice the brightness, twice the contrast).

As shown in Table \ref{tab:corrupt}, we observe that Gaussian noise with a small $\sigma$, changing brightness, and changing contrast force each block to have high similarity after entropy minimization. We find that there are degraded adaptation performances with these selected blocks (e.g., 10.4 $\rightarrow$ 70.8 error rates for CIFAR10-C gradual benchmark with blocks selected by Gaussian noise with 0.1 $\sigma$). We argue that if we use a large enough $\sigma$ compared to the training images' standard deviation (i.e., about 0.45 for CIFAR10 images), we can select blocks that do not lead to error accumulation, and the model's domain-specific feature extraction can be well-adjusted during test-time. On the contrary, when we use relatively simple corruption such as brightness and contrast, the domain-specific features do not differ much from the original source domain, so our block selection cannot work well for finding blocks that are involved in domain-specific feature extraction.

\begin{table}[ht]
\centering
\resizebox{0.5\textwidth}{!}{
\begin{tabular}{lcccccccccccc}
\hline
\multicolumn{1}{c}{}                              & \multicolumn{12}{c}{Blocks}                                                                                                                                                                                                                                                                                                       \\ \cline{2-13} 
\multicolumn{1}{c}{\multirow{-2}{*}{Corruptions}} & 1                            & 2                            & 3                            & 4                            & 5                            & 6                            & 7                            & 8                            & 9                            & 10   & 11                           & 12   \\ \hline
\multicolumn{1}{l|}{GN (0, 0.1)}      & \cellcolor[HTML]{C0C0C0}1.00 & \cellcolor[HTML]{C0C0C0}1.00 & \cellcolor[HTML]{C0C0C0}1.00 & \cellcolor[HTML]{C0C0C0}1.00 & \cellcolor[HTML]{C0C0C0}0.98 & \cellcolor[HTML]{C0C0C0}0.95 & \cellcolor[HTML]{C0C0C0}0.94 & \cellcolor[HTML]{C0C0C0}0.90 & 0.22                         & 0.00 & 0.19                         & 0.22 \\
\multicolumn{1}{l|}{GN (0, 0.5)}      & \cellcolor[HTML]{C0C0C0}0.89 & \cellcolor[HTML]{C0C0C0}0.92 & \cellcolor[HTML]{C0C0C0}1.00 & \cellcolor[HTML]{C0C0C0}0.98 & 0.49                         & 0.47                         & 0.54                         & 0.49                         & 0.30                         & 0.20 & 0.09                         & 0.00 \\
\multicolumn{1}{l|}{GN (0, 1.0)}      & \cellcolor[HTML]{C0C0C0}0.86 & \cellcolor[HTML]{C0C0C0}0.82 & \cellcolor[HTML]{C0C0C0}0.92 & \cellcolor[HTML]{C0C0C0}1.00 & 0.60                         & 0.41                         & 0.31                         & 0.49                         & 0.19                         & 0.37 & 0.00                         & 0.02 \\
\multicolumn{1}{l|}{Brightness}                   & \cellcolor[HTML]{C0C0C0}1.00 & \cellcolor[HTML]{C0C0C0}1.00 & \cellcolor[HTML]{C0C0C0}1.00 & \cellcolor[HTML]{C0C0C0}1.00 & \cellcolor[HTML]{C0C0C0}0.99 & \cellcolor[HTML]{C0C0C0}0.99 & \cellcolor[HTML]{C0C0C0}1.00 & \cellcolor[HTML]{C0C0C0}1.00 & 0.22                         & 0.00 & 0.29                         & 0.10 \\
\multicolumn{1}{l|}{Contrast}                     & \cellcolor[HTML]{C0C0C0}1.00 & \cellcolor[HTML]{C0C0C0}1.00 & \cellcolor[HTML]{C0C0C0}1.00 & \cellcolor[HTML]{C0C0C0}1.00 & \cellcolor[HTML]{C0C0C0}1.00 & \cellcolor[HTML]{C0C0C0}1.00 & \cellcolor[HTML]{C0C0C0}1.00 & \cellcolor[HTML]{C0C0C0}1.00 & \cellcolor[HTML]{C0C0C0}0.92 & 0.00 & \cellcolor[HTML]{C0C0C0}0.83 & 0.28 \\ \bottomrule
\end{tabular}}
\caption{Block selection results with various corruption setting. The block with grey background color is selected. Also, GN ($a$, $b$) refers to the Gaussian noise with $a$ mean and $b$ standard deviation. The block selection is conducted for CIFAR10-C with WRN28-10.}
\label{tab:corrupt}
\end{table}

\begin{figure}[ht!]
    \centering
    \includegraphics[width=0.49\textwidth]{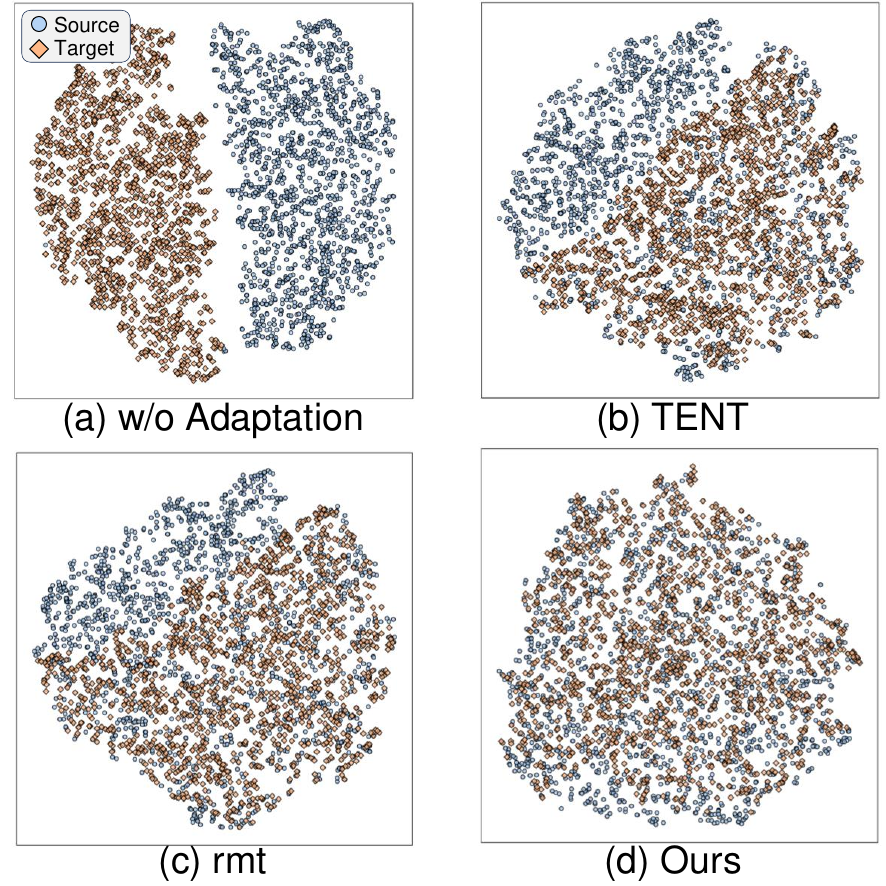}
    \caption{Visualization of features for given original source images (blue) and given Gaussian noise images (orange) produced from the first block of WRN28-10 after adaptation.}
    \label{fig:fv}
\end{figure}

\section*{Domain-specific feature visualization}
We provide feature visualizations of the selected blocks (i.e., block 1-4 of WRN28-10) after adaptation in Figure \ref{fig:fv}. In the experiment, we use the network checkpoint after adaptation on Gaussian noise domain with TENT (b), RMT (c), and Ours (d). Subsequently, we extract features from the source test data and Gaussian noise-added test data, and visualize them using the t-SNE method. Since we specifically train the blocks that are involved in domain-specific feature extraction, source features and target features appear to be well mixed, which can be interpreted as the domain-specific feature extraction being well adjusted. Thus, it demonstrates that our method can outperform other methods when the given test data is corrupted by noise, as shown in Table \ref{tab:cifar10c}.

\begin{table}[t]
\centering
\resizebox{0.35\textwidth}{!}{%
\begin{tabular}{@{}lcccc@{}}
\toprule
Arch.     & Ours & Ours w/ jigsaw & \cite{Yu_2023_CVPR} & \cite{prasanna2023continual} \\ \midrule
WRN28-10  & \textbf{13.7} &  63.5  & 16.4 & 14.3      \\
ResNet18A & \textbf{8.7}  &  9.0        & 10.6 &    9.5   \\ \bottomrule
\end{tabular}}
\caption{Mean classification error rate (\%; $\downarrow$) comparison with the selected block with \cite{Yu_2023_CVPR} or \cite{prasanna2023continual} on CIFAR10-C continual setting benchmark. The best result is indicated in \textbf{bold}.}
\label{tab:blockselect}
\end{table}
\section*{Comparison with other block selection}
Table~\ref{tab:blockselect} provides performance comparison results with selected blocks using three methods: (1) ours w/ jigsaw, using our block selection with jigsaw puzzles as in \cite{Yu_2023_CVPR}, (2) \cite{Yu_2023_CVPR}, using block selection for OOD detection of \cite{Yu_2023_CVPR} (i.e., penultimate block), and (3) \cite{prasanna2023continual}, using selected weights by L1-pruning (40\% ratio as in \cite{prasanna2023continual}). Our block selection outperforms others since \cite{Yu_2023_CVPR} and \cite{prasanna2023continual} use selection method for other task (OOD detection and Pruning), and cannot conduct domain-specific entropy minimization.

\begin{table}[t]
\centering
\resizebox{0.4\textwidth}{!}{%
\begin{tabular}{@{}lccccccc@{}}
\toprule
           & Source & TENT & EATA & CoTTA & RMT & Ours\\ \midrule
Error rate & 88.1   &  91.2  & 73.1 & 73.4  &  77.9     & \textbf{72.5}      \\ \bottomrule
\end{tabular}}
\caption{Mean classification error rate (\%; $\downarrow$) comparison with VGG11-BN on ImageNet-C continual setting benchmark.}
\label{tab:non-residual}
\end{table}

\section*{Evaluation on non-residual network}
We report the adaptation performance when using VGG11-BN, a non-residual network pre-trained on ImageNet provided by PyTorch, in Table \ref{tab:non-residual}. We use VGG11-BN over VGG11 since entropy minimization methods (e.g., TENT, EATA) require BN layers. As VGG does not have blocks, we perform layer-wise selection instead of block-wise selection. Table \ref{tab:non-residual} shows that our method works well for a non-residual network.

\begin{table}[t]
\centering
\resizebox{0.48\textwidth}{!}{
\begin{tabular}{@{}lccccccccc@{}}
\toprule
Time                             & \multicolumn{8}{c}{t$\longrightarrow$}                                                                                                                                                                                  &                       \\ \midrule
\multicolumn{1}{l|}{Round}       & \multicolumn{4}{c|}{1}                                                                                     & \multicolumn{4}{c|}{10}                                                                                    & \multirow{2}{*}{Mean} \\ \cmidrule(r){1-9}
\multicolumn{1}{l|}{Condition}   & \multicolumn{1}{l}{fog} & \multicolumn{1}{l}{night} & \multicolumn{1}{l}{rain} & \multicolumn{1}{l|}{snow} & \multicolumn{1}{l}{fog} & \multicolumn{1}{l}{night} & \multicolumn{1}{l}{rain} & \multicolumn{1}{l|}{snow} &                       \\ \midrule
\multicolumn{1}{l|}{Source}      & 58.1                    & 17.4                      & 42.7                     & \multicolumn{1}{c|}{41.7} & 58.1                    & 17.4                      & 42.7                     & \multicolumn{1}{c|}{41.7} & 40.0                  \\
\multicolumn{1}{l|}{TENT}        &  \textbf{61.1}                    & 20.0                      & 38.1                     & \multicolumn{1}{c|}{35.5} & 5.8                     & 1.0                       & 6.6                      & \multicolumn{1}{c|}{6.7}  & 10.1                  \\
\multicolumn{1}{l|}{CoTTA}       &  60.8                    & 19.6                      & 47.1                     & \multicolumn{1}{c|}{47.1} & 58.3                    & 20.6                      & 45.0                     & \multicolumn{1}{c|}{43.6} & 43.5                  \\
\multicolumn{1}{l|}{PLOT (ours)} & 60.5                    &  \textbf{20.3}                      &  \textbf{47.9}                     & \multicolumn{1}{c|}{ \textbf{50.6}} &  \textbf{59.4}                    &  \textbf{25.8}                      &  \textbf{50.1}                     & \multicolumn{1}{c|}{ \textbf{49.1}} & \textbf{46.4}                  \\ \bottomrule
\end{tabular}}
\caption{Semantic segmentation results (mIoU in \%) on the Cityscapes-to-ACDC online continual test-time adaptation task, where the segmentation model is trained on sunny Cityscapes data and evaluated on the adverse weather ACDC data.}
\label{tab:acdc}
\end{table}
\section*{Extension to segmentation}
Cityscpaes-to-ACDC is a continual semantic segmentation task designed to evaluate the model's robustness against to distribution shifts in the real world. The source model is an off-the-shelf pre-trained segmentation model trained on the Cityscapes dataset \cite{Cordts2016Cityscapes}. Then, the target domains are four adverse visual conditions, including Fog, Night, Rain, and Snow, from the Adverse Conditions Dataset (ACDC) \cite{SDV21}. The ACDC dataset contains images share the same semantic class with Cityscapes. Following \cite{wang2022continual, choi2022improving}, we evaluate the model for the given 10 times-repeated sequence group (i.e., in total 40: fog$\rightarrow$night$\rightarrow$rain$\rightarrow$snow$\rightarrow$fog$\rightarrow$...$\rightarrow$snow) to demonstrate long-term performance and robustness agains to error accumulation.

Specifically, we utilize a ResNet50-based DeepLabV3+ \cite{chen2018encoder} model pre-trained on Cityscapes. Since only CoTTA and TENT apply their methods and open their code to the segmentation task, we compare our method with theirs. The multi-scaling (scale factor of [0.5, 0.75, 1.0, 1.25, 1.5, 1.75, 2.0]) input with flip is used for generating CoTTA's pseudo-label, while we only use horizontal flip for our pseudo-label. We use down-sampled resolutions of 769$\times$769 as inputs to the network and evaluated under the original resolution of 1920$\times$1080. Also, We use Adam optimizer with the learning rate 8 times smaller than the default one and batch size of 1. It is worth noting that we use the first block to adjust domain-specific feature extraction without using block selection. Since the image for segmentation has multiple object class, the output feature of the model cannot be directly used for generating prototype vectors. Instead, as the first block is selected across various architectures in classification tasks, we select the first block (which is named as "stem" in Pytorch implementation).

The experimental results are summarized in Table \ref{tab:acdc}. It is demonstrated that our framework with pseudo-label generated by paired-view is also effective for semantic segmentation tasks. Noticeably, TENT method outperforms other methods in Fog domain of first round, but subsequently, suffers from the error accumulation.
